# Supplementary material for: Geometric direct minimization for low-spin restricted open-shell Hartree-Fock
Source: arXiv:2507.23127 ancillary file (2025-08-04)
Supplement: Supplementary file 1 [file supporting_information.pdf]

# Geometric direct minimization for low-spin restricted open-shell Hartree–Fock: Supplementary Material

Hugh G. A. Burton*
*Department of Chemistry, University College London, London, WC1H 0AJ, U.K.*
(Dated: August 4, 2025)

## S1. GEOMETRY OPTIMIZATION FOR HEXA-AQUO COMPLEXES

Geometry optimization for the $[V(H_2O)_6]^{2+}$, $[Cr(H_2O)_6]^{3+}$, $[Mn(H_2O)_6]^{2+}$, $[Fe(H_2O)_6]^{3+}$, and $[Ni(H_2O)_6]^{2+}$ complexes was performed using ORCA 6.0.[1] The BP86 functional was used with the def2-SVP basis set and the def2/J auxiliary basis set was used to approximate the Coulomb integrals with the RI-J approach. The standard "tight" convergence criteria for geometry optimization were used. Converged geometries are listed below, with coordinates provided in angstroms, and were used for all subsequent calculations with the same metal centre regardless of the oxidation state or spin coupling.

### S1.1. $[V(H_2O)_6]^{2+}$

```
V    0.000000    0.000000    0.000000
O    2.139821   -0.000001    0.000000
O   -2.139821    0.000001    0.000001
O   -0.000002    2.139534    0.000000
O    0.000002   -2.139534    0.000000
O    0.000000   -0.000001   -2.139594
O    0.000000    0.000000    2.139594
H    2.726238    0.783230    0.000000
H    2.726236   -0.783233    0.000000
H    0.000000    2.725892   -0.783273
H    0.000000    2.725892    0.783273
H   -0.783240    0.000001    2.726001
H    0.783241    0.000000    2.726001
H   -2.726237    0.783232    0.000001
H   -2.726238   -0.783231    0.000000
H    0.000000   -2.725891    0.783273
H    0.000000   -2.725892   -0.783273
H   -0.783241    0.000000   -2.726001
H    0.783240    0.000000   -2.726001
```

### S1.2. $[Cr(H_2O)_6]^{3+}$

```
Cr   0.000000    0.000000    0.000000
O    2.002561    0.000000    0.000000
O   -2.002561    0.000000    0.000001
O   -0.000001    2.002561    0.000000
O    0.000000   -2.002561    0.000000
O    0.000000    0.000000   -2.002561
O    0.000000    0.000000    2.002561
H    2.584133    0.799039   -0.000001
H    2.584131   -0.799040    0.000000
H    0.000000    2.584132   -0.799039
H   -0.000001    2.584132    0.799039
H   -0.799039    0.000000    2.584132
H    0.799039    0.000000    2.584132
H   -2.584132    0.799040    0.000000
H   -2.584132   -0.799039    0.000001
H    0.000000   -2.584132    0.799039
```

| | | | |
|---|---|---|---|
| H | 0.000000 | -2.584132 | -0.799039 |
| H | -0.799039 | 0.000000 | -2.584132 |
| H | 0.799039 | 0.000000 | -2.584132 |

### S1.3. $[Mn(H_2O)_6]^{2+}$

| | | | |
|---|---|---|---|
| Mn | 0.000000 | 0.000000 | 0.000000 |
| O | 2.193894 | -0.000001 | 0.000000 |
| O | -2.193894 | 0.000001 | 0.000001 |
| O | -0.000001 | 2.193820 | 0.000000 |
| O | 0.000001 | -2.193820 | 0.000000 |
| O | 0.000000 | 0.000000 | -2.193836 |
| O | 0.000000 | 0.000000 | 2.193836 |
| H | 2.785620 | 0.780200 | 0.000000 |
| H | 2.785618 | -0.780203 | 0.000000 |
| H | -0.000001 | 2.785543 | -0.780204 |
| H | -0.000001 | 2.785543 | 0.780203 |
| H | -0.780204 | 0.000001 | 2.785559 |
| H | 0.780204 | 0.000000 | 2.785559 |
| H | -2.785619 | 0.780203 | 0.000001 |
| H | -2.785620 | -0.780201 | 0.000001 |
| H | 0.000001 | -2.785543 | 0.780203 |
| H | 0.000001 | -2.785543 | -0.780203 |
| H | -0.780204 | 0.000000 | -2.785559 |
| H | 0.780204 | 0.000000 | -2.785559 |

### S1.4. Optimized $[Fe(H_2O)_6]^{3+}$ geometry

| | | | |
|---|---|---|---|
| Fe | 0.000000 | 0.000000 | 0.000000 |
| O | 2.070726 | 0.000000 | 0.000000 |
| O | -2.070726 | 0.000000 | 0.000000 |
| O | 0.000000 | 2.070719 | 0.000000 |
| O | 0.000000 | -2.070719 | 0.000000 |
| O | 0.000000 | 0.000000 | -2.070721 |
| O | 0.000000 | 0.000000 | 2.070721 |
| H | 2.665655 | 0.790685 | -0.000001 |
| H | 2.665654 | -0.790686 | 0.000000 |
| H | -0.000001 | 2.665646 | -0.790685 |
| H | 0.000000 | 2.665646 | 0.790684 |
| H | -0.790685 | 0.000000 | 2.665648 |
| H | 0.790685 | 0.000000 | 2.665648 |
| H | -2.665654 | 0.790686 | 0.000000 |
| H | -2.665655 | -0.790685 | 0.000000 |
| H | 0.000000 | -2.665646 | 0.790685 |
| H | 0.000000 | -2.665647 | -0.790684 |
| H | -0.790685 | 0.000001 | -2.665648 |
| H | 0.790685 | 0.000000 | -2.665648 |

### S1.5. $[Ni(H_2O)_6]^{2+}$

| | | | |
|---|---|---|---|
| Ni | 0.000000 | 0.000000 | 0.000000 |
| O | 2.064359 | 0.000001 | -0.000001 |
| O | -2.064359 | -0.000001 | 0.000001 |
| O | -0.000004 | 2.064331 | 0.000000 |
| O | 0.000004 | -2.064331 | 0.000000 |

```
O    0.000000    -0.000001    -2.064338
O    0.000000     0.000000     2.064338
H    2.644667     0.787697     0.000000
H    2.644666    -0.787696     0.000000
H    0.000003     2.644638    -0.787698
H    0.000002     2.644638     0.787698
H   -0.787697     0.000002     2.644644
H    0.787698    -0.000001     2.644644
H   -2.644667     0.787696     0.000000
H   -2.644667    -0.787697     0.000000
H   -0.000003    -2.644637     0.787698
H   -0.000002    -2.644637    -0.787698
H   -0.787698     0.000002    -2.644644
H    0.787698    -0.000001    -2.644644
```

## S2. GEOMETRY OPTIMIZATION FOR POLYACENE CHAINS

Geometries for the polyacenes with 2–6, 8, 10, and 12 rings were taken from Ref. 2. The remaining structures were obtained through geometry optimization using the UB3LYP functional and the 6-13G(d) basis set with the Q-Chem package.[3] Stability analysis was performed to ensure that the UB3LYP energy corresponds to a local minimum, and the default convergence criteria for geometry optimization was used. The optimized structures are listed below, with coordinates provided in angstroms.

### S2.1. 7-acene

```
C   8.598051  -0.713594   0.000000
C   8.598051   0.713594   0.000000
H   9.544277   1.247513   0.000000
H   9.544277  -1.247513   0.000000
C   7.416797  -1.407835   0.000000
C   7.416797   1.407835   0.000000
C   6.159793  -0.724824   0.000000
C   6.159793   0.724824   0.000000
H   7.414608  -2.495357   0.000000
H   7.414608   2.495357   0.000000
C   4.939989  -1.406488   0.000000
C   4.939989   1.406488   0.000000
C   3.704987  -0.728255   0.000000
C   3.704987   0.728255   0.000000
H   4.940732  -2.494698   0.000000
H   4.940732   2.494698   0.000000
C   2.472632  -1.409137   0.000000
C   2.472632   1.409137   0.000000
C   1.242656  -0.731128   0.000000
C   1.242656   0.731128   0.000000
H   2.473609  -2.497179   0.000000
H   2.473609   2.497179   0.000000
C   0.009742  -1.410171   0.000000
C   0.009742   1.410171   0.000000
C  -1.223114  -0.731155   0.000000
C  -1.223114   0.731155   0.000000
H   0.009789  -2.498177   0.000000
H   0.009789   2.498177   0.000000
C  -2.453118  -1.409158   0.000000
C  -2.453118   1.409158   0.000000
C  -3.685509  -0.728309   0.000000
```

| | | | |
|---|---|---|---|
| C | -3.685509 | 0.728309 | 0.000000 |
| H | -2.454064 | -2.497200 | 0.000000 |
| H | -2.454064 | 2.497200 | 0.000000 |
| C | -4.920420 | -1.406463 | 0.000000 |
| C | -4.920420 | 1.406463 | 0.000000 |
| C | -6.140395 | -0.724878 | 0.000000 |
| C | -6.140395 | 0.724878 | 0.000000 |
| H | -4.921321 | -2.494676 | 0.000000 |
| H | -4.921321 | 2.494676 | 0.000000 |
| C | -7.397199 | -1.407872 | 0.000000 |
| C | -7.397199 | 1.407872 | 0.000000 |
| C | -8.578512 | -0.713548 | 0.000000 |
| C | -8.578512 | 0.713548 | 0.000000 |
| H | -7.395399 | -2.495429 | 0.000000 |
| H | -7.395399 | 2.495429 | 0.000000 |
| H | -9.525064 | -1.247176 | 0.000000 |
| H | -9.525064 | 1.247176 | 0.000000 |

## S2.2. 9-acene

| | | | |
|---|---|---|---|
| H | 12.000646 | -1.247010 | 0.000000 |
| H | 12.000646 | 1.247010 | 0.000000 |
| C | 11.054341 | 0.712944 | 0.000000 |
| C | 11.054341 | -0.712944 | 0.000000 |
| C | 9.872162 | 1.407305 | 0.000000 |
| C | 9.872162 | -1.407305 | 0.000000 |
| C | 8.616735 | 0.724027 | 0.000000 |
| C | 8.616735 | -0.724027 | 0.000000 |
| H | 9.870303 | 2.494863 | 0.000000 |
| H | 9.870303 | -2.494863 | 0.000000 |
| C | 7.394490 | 1.405726 | 0.000000 |
| C | 7.394490 | -1.405726 | 0.000000 |
| C | 6.162823 | 0.727294 | 0.000000 |
| C | 6.162823 | -0.727294 | 0.000000 |
| H | 7.395389 | 2.493951 | 0.000000 |
| H | 7.395389 | -2.493951 | 0.000000 |
| C | 4.925792 | 1.408213 | 0.000000 |
| C | 4.925792 | -1.408213 | 0.000000 |
| C | 3.701327 | 0.730369 | 0.000000 |
| C | 3.701327 | -0.730369 | 0.000000 |
| H | 4.926851 | 2.496288 | 0.000000 |
| H | 4.926851 | -2.496288 | 0.000000 |
| C | 2.461768 | 1.409364 | 0.000000 |
| C | 2.461768 | -1.409364 | 0.000000 |
| C | 1.234362 | 0.731717 | 0.000000 |
| C | 1.234362 | -0.731717 | 0.000000 |
| H | 2.462201 | 2.497416 | 0.000000 |
| H | 2.462201 | -2.497416 | 0.000000 |
| C | -0.000003 | 1.409586 | 0.000000 |
| C | -0.000003 | -1.409586 | 0.000000 |
| C | -1.234368 | 0.731717 | 0.000000 |
| C | -1.234368 | -0.731717 | 0.000000 |
| H | -0.000003 | 2.497638 | 0.000000 |
| H | -0.000003 | -2.497638 | 0.000000 |
| C | -2.461774 | 1.409364 | 0.000000 |
| C | -2.461774 | -1.409364 | 0.000000 |
| C | -3.701333 | 0.730369 | 0.000000 |

| | | | |
|---|---|---|---|
| C | -3.701333 | -0.730369 | 0.000000 |
| H | -2.462207 | 2.497416 | 0.000000 |
| H | -2.462207 | -2.497416 | 0.000000 |
| C | -4.925797 | 1.408214 | 0.000000 |
| C | -4.925797 | -1.408214 | 0.000000 |
| C | -6.162828 | 0.727294 | 0.000000 |
| C | -6.162828 | -0.727294 | 0.000000 |
| H | -4.926857 | 2.496289 | 0.000000 |
| H | -4.926857 | -2.496289 | 0.000000 |
| C | -7.394495 | 1.405726 | 0.000000 |
| C | -7.394495 | -1.405726 | 0.000000 |
| C | -8.616739 | 0.724027 | 0.000000 |
| C | -8.616739 | -0.724027 | 0.000000 |
| H | -7.395394 | 2.493951 | 0.000000 |
| H | -7.395394 | -2.493951 | 0.000000 |
| C | -9.872166 | 1.407306 | 0.000000 |
| C | -9.872166 | -1.407306 | 0.000000 |
| C | -11.054345 | 0.712944 | 0.000000 |
| C | -11.054345 | -0.712944 | 0.000000 |
| H | -9.870308 | 2.494863 | 0.000000 |
| H | -9.870308 | -2.494863 | 0.000000 |
| H | -12.000651 | 1.247009 | 0.000000 |
| H | -12.000651 | -1.247009 | 0.000000 |

### S2.3. 11-acene

| | | | |
|---|---|---|---|
| H | 14.470733 | -1.247046 | 0.000000 |
| H | 14.470733 | 1.247046 | 0.000000 |
| C | 13.524261 | 0.713284 | 0.000000 |
| C | 13.524261 | -0.713284 | 0.000000 |
| C | 12.342619 | 1.407546 | 0.000000 |
| C | 12.342619 | -1.407546 | 0.000000 |
| C | 11.086521 | 0.724289 | 0.000000 |
| C | 11.086521 | -0.724289 | 0.000000 |
| H | 12.340623 | 2.495103 | 0.000000 |
| H | 12.340623 | -2.495103 | 0.000000 |
| C | 9.865235 | 1.405847 | 0.000000 |
| C | 9.865235 | -1.405847 | 0.000000 |
| C | 8.632906 | 0.727261 | 0.000000 |
| C | 8.632906 | -0.727261 | 0.000000 |
| H | 9.865881 | 2.494068 | 0.000000 |
| H | 9.865881 | -2.494068 | 0.000000 |
| C | 7.396470 | 1.408128 | 0.000000 |
| C | 7.396470 | -1.408128 | 0.000000 |
| C | 6.172491 | 0.730023 | 0.000000 |
| C | 6.172491 | -0.730023 | 0.000000 |
| H | 7.397399 | 2.496210 | 0.000000 |
| H | 7.397399 | -2.496210 | 0.000000 |
| C | 4.931826 | 1.409062 | 0.000000 |
| C | 4.931826 | -1.409062 | 0.000000 |
| C | 3.707288 | 0.731180 | 0.000000 |
| C | 3.707288 | -0.731180 | 0.000000 |
| H | 4.932280 | 2.497131 | 0.000000 |
| H | 4.932280 | -2.497131 | 0.000000 |
| C | 2.468996 | 1.409010 | 0.000000 |
| C | 2.468996 | -1.409010 | 0.000000 |
| C | 1.240270 | 0.731381 | 0.000000 |

| | | | |
|---|---|---|---|
| C | 1.240270 | -0.731381 | 0.000000 |
| H | 2.469118 | 2.497098 | 0.000000 |
| H | 2.469118 | -2.497098 | 0.000000 |
| C | 0.006588 | 1.408865 | 0.000000 |
| C | 0.006588 | -1.408865 | 0.000000 |
| C | -1.227069 | 0.731380 | 0.000000 |
| C | -1.227069 | -0.731380 | 0.000000 |
| H | 0.006593 | 2.496965 | 0.000000 |
| H | 0.006593 | -2.496965 | 0.000000 |
| C | -2.455818 | 1.409011 | 0.000000 |
| C | -2.455818 | -1.409011 | 0.000000 |
| C | -3.694090 | 0.731182 | 0.000000 |
| C | -3.694090 | -0.731182 | 0.000000 |
| H | -2.455923 | 2.497099 | 0.000000 |
| H | -2.455923 | -2.497099 | 0.000000 |
| C | -4.918639 | 1.409066 | 0.000000 |
| C | -4.918639 | -1.409066 | 0.000000 |
| C | -6.159305 | 0.730035 | 0.000000 |
| C | -6.159305 | -0.730035 | 0.000000 |
| H | -4.919071 | 2.497135 | 0.000000 |
| H | -4.919071 | -2.497135 | 0.000000 |
| C | -7.383267 | 1.408137 | 0.000000 |
| C | -7.383267 | -1.408137 | 0.000000 |
| C | -8.619730 | 0.727273 | 0.000000 |
| C | -8.619730 | -0.727273 | 0.000000 |
| H | -7.384206 | 2.496219 | 0.000000 |
| H | -7.384206 | -2.496219 | 0.000000 |
| C | -9.852019 | 1.405843 | 0.000000 |
| C | -9.852019 | -1.405843 | 0.000000 |
| C | -11.073340 | 0.724286 | 0.000000 |
| C | -11.073340 | -0.724286 | 0.000000 |
| H | -9.852753 | 2.494069 | 0.000000 |
| H | -9.852753 | -2.494069 | 0.000000 |
| C | -12.329416 | 1.407561 | 0.000000 |
| C | -12.329416 | -1.407561 | 0.000000 |
| C | -13.511056 | 0.713250 | 0.000000 |
| C | -13.511056 | -0.713250 | 0.000000 |
| H | -12.327495 | 2.495115 | 0.000000 |
| H | -12.327495 | -2.495115 | 0.000000 |
| H | -14.457524 | 1.247027 | 0.000000 |
| H | -14.457524 | -1.247027 | 0.000000 |

### S2.4. 13-acene

| | | | |
|---|---|---|---|
| C | 15.976660 | -0.713365 | 0.000000 |
| C | 15.976660 | 0.713365 | 0.000000 |
| H | 16.923169 | 1.247063 | 0.000000 |
| H | 16.923169 | -1.247063 | 0.000000 |
| C | 14.795141 | -1.407662 | 0.000000 |
| C | 14.795141 | 1.407662 | 0.000000 |
| C | 13.538840 | -0.724341 | 0.000000 |
| C | 13.538840 | 0.724341 | 0.000000 |
| H | 14.793290 | 2.495302 | 0.000000 |
| H | 14.793290 | -2.495302 | 0.000000 |
| C | 12.318046 | -1.405994 | 0.000000 |
| C | 12.318046 | 1.405994 | 0.000000 |
| C | 11.085325 | -0.727400 | 0.000000 |

| | | | |
|---|---|---|---|
| C | 11.085325 | 0.727400 | 0.000000 |
| H | 12.318781 | -2.494201 | 0.000000 |
| H | 12.318781 | 2.494201 | 0.000000 |
| C | 9.849434 | -1.408234 | 0.000000 |
| C | 9.849434 | 1.408234 | 0.000000 |
| C | 8.624899 | -0.730085 | 0.000000 |
| C | 8.624899 | 0.730085 | 0.000000 |
| H | 9.850333 | -2.496313 | 0.000000 |
| H | 9.850333 | 2.496313 | 0.000000 |
| C | 7.384905 | -1.409142 | 0.000000 |
| C | 7.384905 | 1.409142 | 0.000000 |
| C | 6.159983 | -0.731072 | 0.000000 |
| C | 6.159983 | 0.731072 | 0.000000 |
| H | 7.385279 | -2.497204 | 0.000000 |
| H | 7.385279 | 2.497204 | 0.000000 |
| C | 4.921911 | -1.408959 | 0.000000 |
| C | 4.921911 | 1.408959 | 0.000000 |
| C | 3.693839 | -0.730980 | 0.000000 |
| C | 3.693839 | 0.730980 | 0.000000 |
| H | 4.921928 | -2.497045 | 0.000000 |
| H | 4.921928 | 2.497045 | 0.000000 |
| C | 2.458833 | -1.408530 | 0.000000 |
| C | 2.458833 | 1.408530 | 0.000000 |
| C | 1.228062 | -0.730702 | 0.000000 |
| C | 1.228062 | 0.730702 | 0.000000 |
| H | 2.458769 | -2.496641 | 0.000000 |
| H | 2.458769 | 2.496641 | 0.000000 |
| C | -0.004674 | -1.408345 | 0.000000 |
| C | -0.004674 | 1.408345 | 0.000000 |
| C | -1.237398 | -0.730702 | 0.000000 |
| C | -1.237398 | 0.730702 | 0.000000 |
| H | -0.004668 | -2.496466 | 0.000000 |
| H | -0.004668 | 2.496466 | 0.000000 |
| C | -2.468181 | -1.408529 | 0.000000 |
| C | -2.468181 | 1.408529 | 0.000000 |
| C | -3.703177 | -0.730981 | 0.000000 |
| C | -3.703177 | 0.730981 | 0.000000 |
| H | -2.468106 | -2.496640 | 0.000000 |
| H | -2.468106 | 2.496640 | 0.000000 |
| C | -4.931260 | -1.408958 | 0.000000 |
| C | -4.931260 | 1.408958 | 0.000000 |
| C | -6.169327 | -0.731074 | 0.000000 |
| C | -6.169327 | 0.731074 | 0.000000 |
| H | -4.931270 | -2.497044 | 0.000000 |
| H | -4.931270 | 2.497044 | 0.000000 |
| C | -7.394254 | -1.409141 | 0.000000 |
| C | -7.394254 | 1.409141 | 0.000000 |
| C | -8.634254 | -0.730090 | 0.000000 |
| C | -8.634254 | 0.730090 | 0.000000 |
| H | -7.394629 | -2.497203 | 0.000000 |
| H | -7.394629 | 2.497203 | 0.000000 |
| C | -9.858780 | -1.408240 | 0.000000 |
| C | -9.858780 | 1.408240 | 0.000000 |
| C | -11.094677 | -0.727383 | 0.000000 |
| C | -11.094677 | 0.727383 | 0.000000 |
| H | -9.859698 | -2.496317 | 0.000000 |
| H | -9.859698 | 2.496317 | 0.000000 |
| C | -12.327367 | -1.405942 | 0.000000 |

```
C -12.327367   1.405942   0.000000
C -13.548358  -0.724401   0.000000
C -13.548358   0.724401   0.000000
H -12.328100  -2.494164   0.000000
H -12.328100   2.494164   0.000000
C -14.804632  -1.407651   0.000000
C -14.804632   1.407651   0.000000
C -15.986127  -0.713341   0.000000
C -15.986127   0.713341   0.000000
H -14.802722  -2.495203   0.000000
H -14.802722   2.495203   0.000000
H -16.932633  -1.247048   0.000000
H -16.932633   1.247048   0.000000
```

### S2.5. 15-acene

```
C  18.435118  -0.713296   0.000000
C  18.435118   0.713296   0.000000
H  19.381694   1.246846   0.000000
H  19.381694  -1.246846   0.000000
C  17.253609  -1.407658   0.000000
C  17.253609   1.407658   0.000000
C  15.997551  -0.724369   0.000000
C  15.997551   0.724369   0.000000
H  17.251820   2.495313   0.000000
H  17.251820  -2.495313   0.000000
C  14.776315  -1.405643   0.000000
C  14.776315   1.405643   0.000000
C  13.543569  -0.727420   0.000000
C  13.543569   0.727420   0.000000
H  14.776900   2.493909   0.000000
H  14.776900  -2.493909   0.000000
C  12.307929  -1.408655   0.000000
C  12.307929   1.408655   0.000000
C  11.083339  -0.730281   0.000000
C  11.083339   0.730281   0.000000
H  12.308693   2.496749   0.000000
H  12.308693  -2.496749   0.000000
C   9.843441  -1.409139   0.000000
C   9.843441   1.409139   0.000000
C   8.618080  -0.731090   0.000000
C   8.618080   0.731090   0.000000
H   9.843344  -2.497151   0.000000
H   9.843344   2.497151   0.000000
C   7.380593  -1.409025   0.000000
C   7.380593   1.409025   0.000000
C   6.151868  -0.730973   0.000000
C   6.151868   0.730973   0.000000
H   7.380588  -2.497105   0.000000
H   7.380588   2.497105   0.000000
C   4.917547  -1.408565   0.000000
C   4.917547   1.408565   0.000000
C   3.686315  -0.730516   0.000000
C   3.686315   0.730516   0.000000
H   4.917411  -2.496670   0.000000
H   4.917411   2.496670   0.000000
C   2.453786  -1.408231   0.000000
```

| | | | |
|---|---|---|---|
| C | 2.453786 | 1.408231 | 0.000000 |
| C | 1.221687 | -0.730212 | 0.000000 |
| C | 1.221687 | 0.730212 | 0.000000 |
| H | 2.453697 | -2.496352 | 0.000000 |
| H | 2.453697 | 2.496352 | 0.000000 |
| C | -0.010466 | -1.408119 | 0.000000 |
| C | -0.010466 | 1.408119 | 0.000000 |
| C | -1.242568 | -0.730214 | 0.000000 |
| C | -1.242568 | 0.730214 | 0.000000 |
| H | -0.010455 | -2.496245 | 0.000000 |
| H | -0.010455 | 2.496245 | 0.000000 |
| C | -2.474720 | -1.408232 | 0.000000 |
| C | -2.474720 | 1.408232 | 0.000000 |
| C | -3.707214 | -0.730522 | 0.000000 |
| C | -3.707214 | 0.730522 | 0.000000 |
| H | -2.474610 | -2.496353 | 0.000000 |
| H | -2.474610 | 2.496353 | 0.000000 |
| C | -4.938482 | -1.408564 | 0.000000 |
| C | -4.938482 | 1.408564 | 0.000000 |
| C | -6.172800 | -0.730978 | 0.000000 |
| C | -6.172800 | 0.730978 | 0.000000 |
| H | -4.938335 | -2.496669 | 0.000000 |
| H | -4.938335 | 2.496669 | 0.000000 |
| C | -7.401528 | -1.409023 | 0.000000 |
| C | -7.401528 | 1.409023 | 0.000000 |
| C | -8.639071 | -0.731127 | 0.000000 |
| C | -8.639071 | 0.731127 | 0.000000 |
| H | -7.401502 | -2.497104 | 0.000000 |
| H | -7.401502 | 2.497104 | 0.000000 |
| C | -9.864402 | -1.409187 | 0.000000 |
| C | -9.864402 | 1.409187 | 0.000000 |
| C | -11.104191 | -0.730134 | 0.000000 |
| C | -11.104191 | 0.730134 | 0.000000 |
| H | -9.864763 | -2.497246 | 0.000000 |
| H | -9.864763 | 2.497246 | 0.000000 |
| C | -12.328838 | -1.408261 | 0.000000 |
| C | -12.328838 | 1.408261 | 0.000000 |
| C | -13.564750 | -0.727393 | 0.000000 |
| C | -13.564750 | 0.727393 | 0.000000 |
| H | -12.329756 | -2.496336 | 0.000000 |
| H | -12.329756 | 2.496336 | 0.000000 |
| C | -14.797401 | -1.405936 | 0.000000 |
| C | -14.797401 | 1.405936 | 0.000000 |
| C | -16.018477 | -0.724379 | 0.000000 |
| C | -16.018477 | 0.724379 | 0.000000 |
| H | -14.798140 | -2.494157 | 0.000000 |
| H | -14.798140 | 2.494157 | 0.000000 |
| C | -17.274688 | -1.407631 | 0.000000 |
| C | -17.274688 | 1.407631 | 0.000000 |
| C | -18.456234 | -0.713311 | 0.000000 |
| C | -18.456234 | 0.713311 | 0.000000 |
| H | -17.272782 | -2.495181 | 0.000000 |
| H | -17.272782 | 2.495181 | 0.000000 |
| H | -19.402726 | -1.247040 | 0.000000 |
| H | -19.402726 | 1.247040 | 0.000000 |

### S2.6. 16-acene

| | | | |
|---|---|---|---|
| C | 19.665641 | -0.713322 | 0.000000 |
| C | 19.665641 | 0.713333 | 0.000000 |
| H | 20.612447 | 1.246530 | 0.000000 |
| H | 20.612446 | -1.246521 | 0.000000 |
| C | 18.484215 | -1.407877 | 0.000000 |
| C | 18.484220 | 1.407894 | 0.000000 |
| C | 17.228134 | -0.724395 | 0.000000 |
| C | 17.228132 | 0.724418 | 0.000000 |
| H | 18.482297 | 2.495609 | 0.000000 |
| H | 18.482243 | -2.495597 | 0.000000 |
| C | 16.006936 | -1.405779 | 0.000000 |
| C | 16.006935 | 1.405805 | 0.000000 |
| C | 14.774037 | -0.727327 | 0.000000 |
| C | 14.774036 | 0.727352 | 0.000000 |
| H | 16.007528 | 2.494130 | 0.000000 |
| H | 16.007527 | -2.494104 | 0.000000 |
| C | 13.538075 | -1.408304 | 0.000000 |
| C | 13.538071 | 1.408327 | 0.000000 |
| C | 12.313429 | -0.730095 | 0.000000 |
| C | 12.313428 | 0.730113 | 0.000000 |
| H | 13.538501 | 2.496438 | 0.000000 |
| H | 13.538514 | -2.496412 | 0.000000 |
| C | 11.073938 | -1.409660 | 0.000000 |
| C | 11.073931 | 1.409671 | 0.000000 |
| C | 9.848506 | -0.731348 | 0.000000 |
| C | 9.848505 | 0.731350 | 0.000000 |
| H | 11.073848 | 2.497718 | 0.000000 |
| H | 11.073874 | -2.497703 | 0.000000 |
| C | 8.610872 | -1.409098 | 0.000000 |
| C | 8.610865 | 1.409091 | 0.000000 |
| C | 7.381998 | -0.730977 | 0.000000 |
| C | 7.381996 | 0.730963 | 0.000000 |
| H | 8.610089 | -2.497128 | 0.000000 |
| H | 8.610075 | 2.497121 | 0.000000 |
| C | 6.147876 | -1.408593 | 0.000000 |
| C | 6.147872 | 1.408575 | 0.000000 |
| C | 4.916332 | -0.730573 | 0.000000 |
| C | 4.916331 | 0.730551 | 0.000000 |
| H | 6.147669 | -2.496708 | 0.000000 |
| H | 6.147662 | 2.496690 | 0.000000 |
| C | 3.684178 | -1.408303 | 0.000000 |
| C | 3.684176 | 1.408279 | 0.000000 |
| C | 2.451707 | -0.730213 | 0.000000 |
| C | 2.451707 | 0.730187 | 0.000000 |
| H | 3.683984 | -2.496424 | 0.000000 |
| H | 3.683980 | 2.496400 | 0.000000 |
| C | 1.219935 | -1.408144 | 0.000000 |
| C | 1.219934 | 1.408118 | 0.000000 |
| C | -0.012296 | -0.730076 | 0.000000 |
| C | -0.012296 | 0.730050 | 0.000000 |
| H | 1.219856 | -2.496268 | 0.000000 |
| H | 1.219855 | 2.496242 | 0.000000 |
| C | -1.244508 | -1.408140 | 0.000000 |
| C | -1.244507 | 1.408115 | 0.000000 |
| C | -2.476293 | -0.730198 | 0.000000 |
| C | -2.476292 | 0.730174 | 0.000000 |

| | | | |
|---|---|---|---|
| H | -1.244455 | -2.496263 | 0.000000 |
| H | -1.244453 | 2.496238 | 0.000000 |
| C | -3.708754 | -1.408288 | 0.000000 |
| C | -3.708752 | 1.408266 | 0.000000 |
| C | -4.940908 | -0.730554 | 0.000000 |
| C | -4.940906 | 0.730535 | 0.000000 |
| H | -3.708591 | -2.496406 | 0.000000 |
| H | -3.708587 | 2.496384 | 0.000000 |
| C | -6.172432 | -1.408613 | 0.000000 |
| C | -6.172429 | 1.408596 | 0.000000 |
| C | -7.406539 | -0.731011 | 0.000000 |
| C | -7.406537 | 0.730998 | 0.000000 |
| H | -6.172227 | -2.496716 | 0.000000 |
| H | -6.172221 | 2.496700 | 0.000000 |
| C | -8.635396 | -1.409051 | 0.000000 |
| C | -8.635392 | 1.409041 | 0.000000 |
| C | -9.872851 | -0.731143 | 0.000000 |
| C | -9.872849 | 0.731138 | 0.000000 |
| H | -8.635307 | -2.497131 | 0.000000 |
| H | -8.635300 | 2.497122 | 0.000000 |
| C | -11.098216 | -1.409198 | 0.000000 |
| C | -11.098212 | 1.409197 | 0.000000 |
| C | -12.337985 | -0.730136 | 0.000000 |
| C | -12.337983 | 0.730139 | 0.000000 |
| H | -11.098510 | -2.497258 | 0.000000 |
| H | -11.098501 | 2.497257 | 0.000000 |
| C | -13.562624 | -1.408262 | 0.000000 |
| C | -13.562619 | 1.408270 | 0.000000 |
| C | -14.798543 | -0.727387 | 0.000000 |
| C | -14.798541 | 0.727400 | 0.000000 |
| H | -13.563480 | -2.496338 | 0.000000 |
| H | -13.563470 | 2.496345 | 0.000000 |
| C | -16.031175 | -1.405930 | 0.000000 |
| C | -16.031170 | 1.405948 | 0.000000 |
| C | -17.252262 | -0.724364 | 0.000000 |
| C | -17.252259 | 0.724385 | 0.000000 |
| H | -16.031872 | -2.494152 | 0.000000 |
| H | -16.031862 | 2.494169 | 0.000000 |
| C | -18.508461 | -1.407615 | 0.000000 |
| C | -18.508455 | 1.407642 | 0.000000 |
| C | -19.690012 | -0.713285 | 0.000000 |
| C | -19.690010 | 0.713317 | 0.000000 |
| H | -18.506533 | -2.495166 | 0.000000 |
| H | -18.506523 | 2.495193 | 0.000000 |
| H | -20.636498 | -1.247025 | 0.000000 |
| H | -20.636493 | 1.247060 | 0.000000 |

## S3. SUPPLEMENTARY RESULTS

TABLE S1: Converged CSF energies ($E_h$) for the hexa-aqua complexes (def2-SVP) using initial orbitals from a converged high-spin ROHF calculation. Solutions that are not the lowest energy for a given structure and spin coupling are highlighted in italics.

| | | CSF-GDM | CSF-GDM (no PC) | CSF-GDM (no PT) | L-BFGS | CSF-ROHF |
|---|---|---|---|---|---|---|
| $[V(H_2O)_6]^{2+}$ | [++−] | −1398.232485 | −1398.232485 | −1398.232485 | −1398.232485 | *−1398.229444* |
| | [+−+] | −1398.232607 | −1398.232607 | −1398.232607 | −1398.232607 | *−1398.229424* |
| $[V(H_2O)_6]^{3+}$ | [+−] | −1397.661357 | −1397.661357 | −1397.661357 | −1397.661357 | −1397.661357 |
| $[Cr(H_2O)_6]^{2+}$ | [++−−] | −1498.463166 | −1498.463166 | −1498.463166 | −1498.463166 | *−1498.460455* |
| | [+−+−] | −1498.476792 | −1498.476792 | −1498.476792 | −1498.476792 | *−1498.460483* |
| | [+++−] | −1498.511263 | −1498.511263 | −1498.511263 | −1498.511263 | −1498.511263 |
| | [++−+] | −1498.516324 | −1498.516324 | −1498.516324 | −1498.516324 | *−1498.504505* |
| | [+−++] | −1498.521138 | −1498.521138 | −1498.521138 | −1498.521138 | *−1498.504351* |
| $[Cr(H_2O)_6]^{3+}$ | [++−] | −1497.983320 | −1497.983320 | −1497.983320 | −1497.983320 | −1497.983320 |
| | [+−+] | −1497.983502 | −1497.983502 | −1497.983502 | −1497.983502 | −1497.983502 |
| $[Mn(H_2O)_6]^{2+}$ | [+++−−] | −1604.961635 | −1604.961635 | −1604.961635 | −1604.961635 | −1604.961635 |
| | [++−+−] | −1604.971353 | −1604.971353 | −1604.971353 | −1604.971353 | *−1604.920283* |
| | [+−++−] | −1604.977578 | −1604.977578 | −1604.977578 | −1604.977578 | *−1604.948127* |
| | [++−−+] | −1604.961448 | −1604.961448 | −1604.961448 | −1604.961448 | *−1604.958641* |
| | [+−+−+] | −1604.976065 | −1604.976065 | −1604.976065 | −1604.976065 | *−1604.930838* |
| | [++++−] | −1605.036258 | −1605.036258 | −1605.036258 | −1605.036258 | −1605.036258 |
| | [+++−+] | −1605.040612 | −1605.040612 | −1605.040612 | −1605.040612 | failed |
| | [++−++] | −1605.047352 | −1605.047352 | −1605.047352 | −1605.047352 | *−1605.035037* |
| | [+−+++] | −1605.049050 | −1605.049050 | −1605.049050 | −1605.049050 | *−1605.034986* |
| $[Fe(H_2O)_6]^{2+}$ | [++−−] | −1717.549602 | −1717.549602 | −1717.549602 | −1717.549602 | *−1717.546928* |
| | [+−+−] | −1717.564968 | −1717.564968 | −1717.564968 | −1717.564968 | *−1717.514983* |
| | [+++−] | −1717.606299 | −1717.606299 | −1717.606299 | −1717.606299 | *−1717.578786* |
| | [++−+] | −1717.613160 | −1717.613160 | −1717.613160 | −1717.613160 | −1717.613160 |
| | [+−++] | −1717.616403 | −1717.616403 | −1717.616403 | −1717.616403 | *−1717.596583* |
| $[Fe(H_2O)_6]^{3+}$ | [+++−−] | −1716.844253 | −1716.844253 | *−1716.843054* | −1716.844253 | *−1716.770637* |
| | [++−+−] | −1716.920870 | −1716.920870 | −1716.920870 | −1716.920870 | −1716.920870 |
| | [+−++−] | −1716.929605 | −1716.929605 | −1716.929605 | −1716.929605 | *−1716.872476* |
| | [++−−+] | −1716.935763 | −1716.935763 | −1716.935763 | −1716.935763 | *−1716.902139* |
| | [+−+−+] | −1716.916441 | −1716.916441 | −1716.916441 | −1716.916441 | *−1716.911895* |
| | [++++−] | −1716.933069 | −1716.933069 | −1716.933069 | −1716.933069 | *−1716.882275* |
| | [+++−+] | −1717.004821 | −1717.004821 | −1717.004821 | −1717.004821 | failed |
| | [++−++] | −1717.008644 | −1717.008644 | −1717.008644 | −1717.008644 | *−1717.008630* |
| | [+−+++] | −1717.013100 | −1717.013100 | −1717.013100 | −1717.013100 | *−1716.994885* |
| $[Ni(H_2O)_6]^{2+}$ | [+−] | −1962.030449 | *−1961.660731* | −1962.030449 | −1962.030449 | −1962.030447 |

TABLE S2: Converged CSF energies ($E_h$) for the hexa-aqua complexes (def2-SVP) starting from a core orbital guess. Solutions that are not the lowest energy for a given structure and spin coupling are highlighted in italics.

| | | CSF-GDM | CSF-GDM (no PC) | CSF-GDM (no PT) | L-BFGS | CSF-ROHF |
|---|---|---|---|---|---|---|
| $[V(H_2O)_6]^{2+}$ | [++−] | −1398.232485 | −1398.232485 | −1398.232485 | −1398.232485 | *−1398.229444* |
| | [+−+] | −1398.232607 | −1398.232607 | −1398.232607 | −1398.232607 | *−1397.684588* |
| $[V(H_2O)_6]^{3+}$ | [+−] | −1397.661360 | *−1397.661357* | *−1397.661357* | *−1397.661357* | *−1397.616299* |
| $[Cr(H_2O)_6]^{2+}$ | [++−−] | −1498.463166 | −1498.463166 | −1498.463166 | −1498.463166 | failed |
| | [+−+−] | −1498.476792 | −1498.476792 | −1498.476792 | *−1498.252800* | failed |
| | [+++−] | *−1498.511263* | −1498.513816 | *−1498.511263* | −1498.513816 | *−1498.449669* |
| | [++−+] | −1498.516324 | −1498.516324 | −1498.516324 | −1498.516324 | *−1498.447991* |
| | [+−++] | −1498.521138 | −1498.521138 | −1498.407759 | −1498.521138 | *−1498.015221* |
| $[Cr(H_2O)_6]^{3+}$ | [++−] | −1497.983320 | −1497.983320 | −1497.983320 | −1497.983320 | *−1497.860372* |
| | [+−+] | −1497.983502 | −1497.983502 | −1497.983502 | −1497.983502 | *−1497.860372* |
| $[Mn(H_2O)_6]^{2+}$ | [+++−−] | *−1604.756201* | −1604.962747 | −1604.962747 | −1604.962747 | *−1604.962290* |
| | [++−+−] | *−1604.688782* | −1604.971353 | *−1604.691008* | *−1604.669074* | *−1604.920283* |
| | [+−++−] | *−1604.725349* | *−1604.688703* | *−1604.724346* | −1604.977678 | *−1604.948127* |
| | [++−−+] | −1604.961448 | *−1604.731984* | *−1604.681743* | *−1604.731858* | *−1604.960656* |
| | [+−+−+] | *−1604.676426* | *−1604.712436* | *−1604.674691* | *−1604.681037* | −1604.958166 |
| | [++++−] | *−1604.741928* | *−1604.697188* | −1605.038799 | −1605.038799 | *−1605.036258* |
| | [+++−+] | *−1604.708976* | *−1604.705059* | −1605.042800 | *−1604.708976* | failed |
| | [++−++] | *−1604.685920* | −1605.047352 | −1605.047352 | *−1604.380856* | *−1605.045298* |
| | [+−+++] | −1605.049050 | −1605.049050 | *−1604.725803* | −1605.049050 | *−1604.604434* |
| $[Fe(H_2O)_6]^{2+}$ | [++−−] | −1717.549602 | *−1717.336750* | *−1717.285303* | *−1717.332764* | *−1717.549338* |
| | [+−+−] | −1717.564967 | −1717.564967 | −1717.564967 | *−1717.315657* | failed |
| | [+++−] | *−1717.322709* | −1717.606299 | −1717.606299 | *−1717.306544* | *−1717.605466* |
| | [++−+] | −1717.613616 | −1717.613616 | −1717.613616 | *−1717.320002* | *−1717.607195* |
| | [+−++] | −1717.616403 | −1717.616403 | −1717.616403 | *−1717.314152* | failed |
| $[Fe(H_2O)_6]^{3+}$ | [+++−−] | −1716.844253 | −1716.844253 | *−1716.843054* | −1716.844253 | *−1716.770637* |
| | [++−+−] | −1716.874681 | −1716.874682 | *−1716.855765* | *−1716.855765* | *−1716.789468* |
| | [+−++−] | −1716.886530 | *−1716.558499* | −1716.886530 | *−1716.850881* | failed |
| | [++−−+] | −1716.870752 | −1716.870751 | −1716.870752 | *−1716.582388* | *−1716.802605* |
| | [+−+−+] | −1716.873332 | *−1716.873015* | *−1716.840773* | *−1716.575707* | failed |
| | [++++−] | −1716.890762 | −1716.890762 | −1716.890762 | −1716.890762 | failed |
| | [+++−+] | −1716.900813 | −1716.900813 | *−1716.587090* | *−1716.597354* | *−1716.807952* |
| | [++−++] | *−1716.595715* | *−1716.911609* | −1716.981844 | *−1716.911978* | *−1716.822176* |
| | [+−+++] | −1717.014072 | *−1716.602559* | −1717.014072 | −1717.014072 | failed |
| $[Ni(H_2O)_6]^{2+}$ | [+−] | −1962.030449 | *−1961.660731* | −1962.030449 | −1962.030449 | −1962.030447 |

TABLE S3: Converged CSF local minima ($E_h$) for the $[Fe(SCH_3)_4]^-$ complex (def2-TZVP) with different spin coupling vectors. Local minima were identified from 100 random starting points for each spin coupling vector, and thus these results are not expected to be exhaustive.

| [+++++] | [++++−] | [+++−+] | [++−++] | [+−+++] | [+++−−] | [++−+−] | [++−−+] | [+−++−] | [+−+−+] |
|---|---|---|---|---|---|---|---|---|---|
| −3011.148027 | −3011.074238 | −3011.067138 | −3011.055969 | −3011.031649 | −3010.961468 | −3010.967074 | −3010.952295 | −3010.967813 | −3010.954751 |
| −3010.817802 | −3010.971925 | −3010.980204 | −3010.991521 | −3011.006582 | −3010.959982 | −3010.957373 | −3010.910967 | −3010.967094 | −3010.954651 |
| | −3010.964410 | −3010.965897 | −3010.989927 | −3010.972206 | −3010.955729 | −3010.939598 | −3010.812140 | −3010.963395 | −3010.954638 |
| | −3010.812503 | −3010.813150 | −3010.971243 | −3010.970167 | −3010.928486 | −3010.939018 | −3010.797844 | −3010.951562 | −3010.936472 |
| | −3010.788247 | −3010.810009 | −3010.806773 | −3010.809986 | −3010.927872 | −3010.923474 | −3010.794186 | −3010.934726 | −3010.936169 |
| | −3010.784887 | −3010.807222 | −3010.806469 | −3010.809619 | −3010.812468 | −3010.923474 | −3010.793118 | −3010.934241 | −3010.924884 |
| | −3010.783940 | −3010.795574 | −3010.805941 | −3010.800403 | −3010.811521 | −3010.807820 | −3010.792962 | −3010.934183 | −3010.797985 |
| | −3010.779942 | −3010.789515 | −3010.794059 | −3010.799407 | −3010.795239 | −3010.793786 | −3010.779037 | −3010.934056 | −3010.797884 |
| | −3010.779377 | −3010.783029 | −3010.779276 | −3010.798940 | −3010.793966 | −3010.790807 | −3010.778955 | −3010.811399 | −3010.797413 |
| | −3010.768639 | −3010.782447 | −3010.778586 | −3010.798760 | −3010.792541 | −3010.789981 | −3010.777849 | −3010.807779 | −3010.797251 |
| | −3010.768597 | −3010.777858 | −3010.777797 | −3010.797610 | −3010.792379 | −3010.789558 | −3010.774317 | −3010.798418 | −3010.795544 |
| | | −3010.775764 | −3010.773131 | −3010.780004 | −3010.792379 | −3010.787054 | −3010.773772 | −3010.797858 | −3010.794592 |
| | | | −3010.772939 | −3010.778958 | −3010.778540 | −3010.781585 | −3010.770331 | −3010.797808 | −3010.792078 |
| | | | | −3010.778580 | −3010.774035 | −3010.780604 | −3010.769867 | −3010.797207 | −3010.778836 |
| | | | | | −3010.769559 | −3010.772729 | −3010.752346 | −3010.796220 | −3010.778211 |
| | | | | | −3010.758251 | −3010.770183 | −3010.752069 | −3010.796137 | −3010.778122 |
| | | | | | −3010.756989 | −3010.769684 | −3010.741951 | −3010.794986 | −3010.778059 |
| | | | | | −3010.752921 | −3010.766241 | | −3010.794972 | −3010.777518 |
| | | | | | −3010.746118 | −3010.756142 | | −3010.780966 | −3010.776498 |
| | | | | | | −3010.750103 | | −3010.780224 | −3010.760867 |
| | | | | | | −3010.740558 | | −3010.780076 | −3010.756526 |
| | | | | | | | | −3010.777359 | |
| | | | | | | | | −3010.776232 | |
| | | | | | | | | −3010.776083 | |
| | | | | | | | | −3010.774821 | |
| | | | | | | | | −3010.774253 | |
| | | | | | | | | −3010.767467 | |

TABLE S4: Converged CSF local minima ($E_h$) for the $[Fe_2S_2(SCH_3)_4]^{2-}$ complex (def2-TZVP) with different spin coupling vectors. Local minima were identified from 100 random starting points for each spin coupling vector, and thus these results are not expected to be exhaustive. The lowest energy minimum for the [+++++−−−−−] CSF was found using a physically motivated initial guess.

| [++++++++++] | [+++++−−−−−] |
|---|---|
| −5068.259547 | −5068.255702 |
| −5068.177090 | −5068.116669 |
| −5068.131590 | −5068.017194 |
| −5068.129961 | −5068.016641 |
| −5067.899013 | −5068.013984 |
| −5067.891197 | −5067.958889 |
| −5067.890807 | −5067.926329 |
| −5067.890349 | −5067.915549 |
| −5067.856266 | −5067.915204 |
| −5067.849373 | −5067.913038 |
| −5067.831287 | −5067.912944 |
| | −5067.898220 |
| | −5067.898205 |
| | −5067.880973 |
| | −5067.880866 |
| | −5067.880700 |
| | −5067.880684 |
| | −5067.880578 |
| | −5067.855703 |
| | −5067.851253 |
| | −5067.851121 |
| | −5067.850536 |
| | −5067.843574 |
| | −5067.840123 |
| | −5067.837030 |
| | −5067.820394 |
| | −5067.817593 |
| | −5067.813364 |
| | −5067.808262 |
| | −5067.779421 |
| | −5067.775166 |
| | −5067.750712 |
| | −5067.748120 |
| | −5067.746993 |
| | −5067.743366 |
| | −5067.741975 |
| | −5067.740841 |
| | −5067.737344 |
| | −5067.736869 |
| | −5067.727692 |
| | −5067.716496 |
| | −5067.713647 |
| | −5067.712966 |
| | −5067.711750 |
| | −5067.709824 |
| | −5067.702642 |
| | −5067.690213 |
| | −5067.689277 |
| | −5067.688770 |
| | −5067.687884 |
| | −5067.685743 |
| | −5067.684540 |
| | −5067.674906 |
| | −5067.673248 |
| | −5067.671300 |
| | −5067.671259 |
| | −5067.660326 |

TABLE S5: Converged singlet CSF energies ($E_h$) for the polyacene chains (cc-pVDZ) with various spin coupling patterns. There is only a small difference between the energies of different CSFs with the same number of unpaired electrons.

| | RHF | [+−] | [+−+−] | [++−−] | [+−+−+−] | [+−++−−] | [++−−+−] | [++−+−−] | [+++−−−] |
|---|---|---|---|---|---|---|---|---|---|
| 2-acene | −383.383583 | −383.259781 | −383.083887 | −383.082226 | −382.903844 | −382.913455 | −382.913455 | −382.905721 | −382.906628 |
| 3-acene | −536.037093 | −535.952807 | −535.767128 | −535.778801 | −535.594626 | −535.592382 | −535.595408 | −535.622700 | −535.597025 |
| 4-acene | −688.686483 | −688.622185 | −688.472769 | −688.471530 | −688.280774 | −688.281562 | −688.281745 | −688.280672 | −688.279787 |
| 5-acene | −841.333548 | −841.290332 | −841.178556 | −841.179320 | −840.970027 | −840.970202 | −840.993109 | −840.970633 | −840.969856 |
| 6-acene | −993.977729 | −993.950342 | −993.859855 | −993.860255 | −993.657053 | −993.656555 | −993.656236 | −993.655825 | −993.655424 |
| 7-acene | −1146.618183 | −1146.610595 | −1146.532579 | −1146.533359 | −1146.413158 | −1146.414972 | −1146.414972 | −1146.415509 | −1146.415579 |
| 8-acene | −1299.259619 | −1299.262734 | −1299.202943 | −1299.200197 | −1299.093123 | −1299.093747 | −1299.094806 | −1299.095246 | −1299.095440 |
| 9-acene | −1451.901606 | −1451.913462 | −1451.862300 | −1451.861945 | −1451.770908 | −1451.771453 | −1451.772303 | −1451.771955 | −1451.772797 |
| 10-acene | −1604.544206 | −1604.560529 | −1604.522174 | −1604.518522 | −1604.440539 | −1604.440992 | −1604.441976 | −1604.442446 | −1604.442649 |
| 11-acene | −1757.187011 | −1757.207126 | −1757.180353 | −1757.181078 | −1757.110486 | −1757.111964 | −1757.111964 | −1757.112595 | −1757.112816 |
| 12-acene | −1909.829803 | −1909.851514 | −1909.833500 | −1909.833924 | −1909.772490 | −1909.773791 | −1909.773791 | −1909.774430 | −1909.773884 |
| 13-acene | −2062.472532 | −2062.495484 | −2062.484845 | −2062.485491 | −2062.433782 | −2062.434015 | −2062.434820 | −2062.435276 | −2062.435406 |
| 14-acene | −2215.115105 | −2215.138320 | −2215.136672 | −2215.136957 | −2215.090703 | −2215.090903 | −2215.091992 | −2215.092715 | −2215.092872 |
| 15-acene | −2367.757749 | −2367.781149 | −2367.785453 | −2367.785516 | −2367.750564 | −2367.750704 | −2367.751521 | −2367.751516 | −2367.752145 |
| 16-acene | −2520.400348 | −2520.423655 | −2520.432267 | −2520.432219 | −2520.404177 | −2520.404282 | −2520.404973 | −2520.404958 | −2520.405478 |

## REFERENCES

---

[*] h.burton@ucl.ac.uk

[1] Neese, F. Software update: The ORCA program system - Version 5.0. *WIREs Comput. Mol. Sci.* **2022**, *12*, e1606.
[2] Hachmann, J.; Dorando, J. J.; Avilés, M.; Chan, G. K.-L. The radical character of the acenes: A density matrix renormalization group study. *J. Chem. Phys.* **2007**, *127*, 134309.
[3] Shao, Y. et al. Advances in molecular quantum chemistry contained in the Q-Chem 4 program package. *Mol. Phys.* **2015**, *113*, 184.
